# Supplementary material for: Motility-induced mixing transition in exponentially growing multicellular spheroids
Source: arXiv:2403.11002 ancillary file (2025-02-10)
Supplement: Supplementary file 1 [file supplement.pdf]

# Supplemental material for
# "Motility-induced mixing transition in exponentially growing multicellular spheroids"

Torben Sunkel,[1,2] Lukas Hupe,[1,2] and Philip Bittihn[1,2,*]

[1] *Max Planck Institute for Dynamics and Self-Organization, Göttingen, Germany*

[2] *Institute for the Dynamics of Complex Systems, Göttingen University, Göttingen, Germany*

## I. AGENT-BASED MODEL

Our agent-based cell model is related to that introduced by Isensee et al [1].

Cells are modeled as three-dimensional dumbbells, consisting of two spheres (nodes) of equal radius $R$ connected by a spring between their centers. To model cell growth and division, each cell has an internal clock $g$ that increases from 0 to 1 with a *growth rate* $\gamma = \frac{\mathrm{d}g}{\mathrm{d}t}$. This *growth progress* sets the rest length of the internal spring $b^{\mathrm{eq}} = 2Rg$: initially, both nodes overlap completely ($b^{\mathrm{eq}} = 0$) and get pushed apart until full separation ($b^{\mathrm{eq}} = 2R$) This extension initially starts along an arbitrary axis $\hat{\mathbf{b}}$, although it can later be reoriented by external interactions.

When $b^{\mathrm{eq}}$ reaches its maximum, the cell divides by replacing the individual nodes with new cells with $b^{\mathrm{eq}} = 0$. New cells are randomly assigned a new director $\hat{\mathbf{b}}$ from a uniform distribution on the 2-sphere, as well as a new growth rate from a uniform distribution on the interval $[\frac{3}{4}, \frac{5}{4}]$. This growth rate randomization helps to prevent excessive synchronization of cell growth cycles. All other parameters are inherited from the parent cell.

### A. Steric forces

In this model, forces act between the individual nodes of different cells (*external forces*) as well as between the individual nodes of a single cell (*internal forces*). External forces are used to model intercellular interactions (steric repulsion, crawling motility), internal forces are used to push the nodes of a growing cell apart. In the following, we use Latin indices for individual cells and Greek indices for their nodes.

The force exerted on a node at position $\mathbf{r}_i^\alpha$ by its steric interaction with a node at position $\mathbf{r}_j^\beta$ is modelled using Hertzian contact theory [2], with

$$\mathbf{F}^{\mathrm{steric}}_{\alpha\beta ij} = m_{ij} \frac{\Upsilon}{2} \sqrt{\frac{R}{2}} \left(2R - \|\mathbf{d}_{\alpha\beta ij}\|\right)^{3/2} \cdot \frac{\mathbf{d}_{\alpha\beta ij}}{\|\mathbf{d}_{\alpha\beta ij}\|} \quad \text{for } i \neq j \text{ and } \|\mathbf{d}_{\alpha\beta ij}\| \leq 2R\,, \tag{1}$$

where $\mathbf{d}_{\alpha\beta ij} = r_i^\alpha - r_j^\beta$ and $\Upsilon$ is the effective Young's modulus of the cells.

The softness factor $m_{ij}$ is introduced to address a problem at cell division: when a single node is replaced with two overlapping nodes, steric forces with a neighbor will double

* philip.bittihn@ds.mpg.de

instantaneously. This issue is treated by scaling all interactions between cells $i$ and $j$ with the factor $m_{i,j} \in \left[\frac{1}{4}, 1\right]$, which reduces forces depending on the cell growth progress:

$$m_{i,j} = \frac{\cdot(1+g_i)\cdot(1+g_j)}{4}\,. \tag{2}$$

To keep the forces in between nodes consistent with intercellular interactions, we also choose a Hertzian-inspired force law for the internal spring:

$$\mathbf{F}^{\text{steric}}_{\alpha\beta ii} = \frac{\Upsilon}{2}\sqrt{\frac{R}{2}}\cdot \text{sgn}(\Delta b_i)\cdot|\Delta b_i|^{3/2}\frac{\mathbf{d}_{\alpha\beta ii}}{\|\mathbf{d}_{\alpha\beta ii}\|}\text{for}\alpha \neq \beta \tag{3}$$

with $\Delta b_i = b_i^{\text{eq}} - b_i$ the compression of the spring.

### B. Motility

In 2D systems, cell motility is usually implemented by letting particles propel along a substrate, which provides the necessary reaction force. This could be expanded to 3D by allowing the cells to swim in their medium. However, here, we are interested in cells that can crawl along the surfaces of their neighbors. To this end, we again introduce a force that scales with node overlap (to model increased crawling effectiveness with increasing contact area), but with the direction of the force determined by the orientation vectors $\mathbf{b}_i$ and $\mathbf{b}_j$ of the cells:

$$\mathbf{F}^{\text{mot}}_{\alpha\beta ij} = m_{ij}\cdot M\cdot(2R - \|\mathbf{d}_{\alpha\beta ij}\|)\cdot(\hat{\mathbf{b}}_i - \hat{\mathbf{b}}_j) \quad \text{for } i \neq j \text{ and } \|\mathbf{d}_{\alpha\beta ij}\| \leq 2R\,. \tag{4}$$

The magnitude of this force is maximal if the cells face in opposite directions, and vanishes if both backbones are parallel, as cells cannot move in the same direction by pushing on each other.

### C. Equations of motion

We want to write the equations of motions for the degrees of freedom of a cell, which are the center of mass $\mathbf{r}^{\text{cm}}$, the node-to-node distance $b$ and orientation $\hat{\mathbf{b}}$. Since forces in this model always act on nodes, we first need to transform the total node forces, which for

a node $\alpha$ of cell $i$ is computed as a sum over all other nodes

$$\mathbf{F}_i^{\alpha} = \sum_{\beta,j} \mathbf{F}_{\alpha\beta ij}^{\text{steric}} + \mathbf{F}_{\alpha\beta ij}^{\text{mot}} \tag{5}$$

into forces acting on the cell degrees of freedom. For this, we designate the nodes as *positive* (+) and *negative* (−), with the orientation vector $\hat{\mathbf{b}}$ defined as pointing from the negative to the positive node position. Dropping the cell index $i$ from the previous section, we can now write the cell forces for a single cell in terms of the total node forces for both nodes

$$\mathbf{F}^{\text{cm}} = \mathbf{F}^{+} + \mathbf{F}^{-} \tag{6}$$

$$F^{\text{int}} = \hat{\mathbf{b}} \cdot (\mathbf{F}^{+} - \mathbf{F}^{-}) \tag{7}$$

$$\mathbf{T} = \frac{b}{2}\hat{\mathbf{b}} \times (\mathbf{F}^{+} - \mathbf{F}^{-}) \tag{8}$$

where $\mathbf{F}^{\text{cm}}$ is the translational force acting on the center of mass, $F^{\text{int}}$ is the force on the node-to-node distance and $\mathbf{T}$ is the torque with respect to the center of mass.

Using overdamped dynamics (i.e., neglecting inertial effects), the equations of motion of a single cell read

$$\frac{\mathrm{d}\mathbf{r}^{\text{cm}}}{\mathrm{d}t} = \underline{\boldsymbol{\mu}}^{\text{cm}}\,\mathbf{F}^{\text{cm}} \tag{9}$$

$$\frac{\mathrm{d}b}{\mathrm{d}t} = \mu^{\text{int}} \cdot F^{\text{int}} \tag{10}$$

$$\frac{\mathrm{d}\hat{\mathbf{b}}}{\mathrm{d}t} = \mu^{\text{rot}} \cdot \mathbf{T} \times \hat{\mathbf{b}}\,, \tag{11}$$

where $\underline{\boldsymbol{\mu}}^{\text{cm}}$ is the translational mobility tensor, $\mu^{\text{int}}$ is the mobility of the internal dynamics, and $\mu^{\text{rot}}$ is the rotational mobility.

For the mobilities, we assume that $\underline{\boldsymbol{\mu}}^{\text{cm}}$ has the eigenvalues $\mu^{\parallel}$ along $\hat{\mathbf{b}}$ and $\mu^{\perp}$ orthogonal to it. We use numerically approximated expressions for the mobility of rods in a viscous

fluid, as derived by Tirado et al. [3–6], with

$$\mu^{\parallel}(a) = \frac{1}{2\pi\eta(2Ra)}\left(\ln(a) - 0.207 + 0.980a^{-1} - 0.133a^{-2}\right) \tag{12}$$

$$\mu^{\perp}(a) = \frac{1}{4\pi\eta(2Ra)}\left(\ln(a) + 0.839 + 0.185a^{-1} - 0.233a^{-2}\right) \tag{13}$$

$$\mu^{\mathrm{rot}}(a) = \frac{3}{\pi\eta(2Ra)^3}\left(\ln(a) - 0.662 + 0.917a^{-1} - 0.050a^{-2}\right), \tag{14}$$

where $a = b/2R + 1$ is the aspect ratio of a cell and $\eta$ is the fluid viscosity. Here, we use $\eta = 0.5$.

To keep the internal degree of freedom of the cell consistent with the center of mass movement, we set $\mu^{\mathrm{int}} = 2\mu^{\parallel}$ (see [7] for a explanation).

### D. Parameters, length and time scales

We choose a Young's modulus of $\Upsilon = 10^5$. For the motility parameter, we investigate the range of $M \in [0, 4000]$.

We set the radius of a node of a cell to 0.5. Then, the maximum extent of a cell along its axis varies from 1 (complete overlap of nodes) to 2 (detached nodes).

We choose the average time between individual cell divisions as the time unit of the simulation, which is then simply measured in generations.

An overview of parameters is shown in Table I.

| | |
|---|---|
| cell diameter $2R$ | 1 |
| viscosity $\eta$ | 0.5 |
| Young's modulus $\Upsilon$ | $10^5$ |
| motility $M$ | 0...4000 |

TABLE I. Parameters used in simulations

## II. THEORETICAL CONSIDERATIONS

### A. Radial expansion

We assume incompressible cells and an isotropic exponential growth with a rate $\alpha$ so that the volume grows like $V(t) = V_0 \exp(\alpha t)$. Also assuming that the colony maintains

its spherical shape, the volume growth can be written in terms of a radial growth: $V(t) = \frac{4}{3}\pi R(t)^3$ where $R(t) = R_0 \exp(\alpha' t)$ and $\alpha' := \frac{\alpha}{3}\ln 2$. Here, $R_0$ denotes the radius at the surface, but due to incompressibility, the expression is also valid for any sphere below. The first time-derivative of the radius yields the radial velocity of the surface *of* a sphere:

$$v_{\mathrm{rad}}(t, R_0) = \frac{\mathrm{d}}{\mathrm{d}t} R(t) = \alpha' R(t) = \alpha' R_0 \exp(\alpha' t) \tag{15}$$

The velocity *in* a fixed sphere at position $r$ is time independent:

$$v_{\mathrm{rad}}(r) = v_{\mathrm{rad}}(t, R_0)\Big|_{R_0=r,\ t=0} = \alpha' r \tag{16}$$

Here, one can easily see the intuitively expected linear dependency of the radial velocity on the radius. To evaluate the time dependency of the average radial velocity $\langle v_{\mathrm{rad}} \rangle_r$, a simple integration can be performed:

$$\langle v_{\mathrm{rad}} \rangle_r(t) = \frac{\int_{V(t)} v_{\mathrm{rad}}(r)\mathrm{d}V}{\int_{V(t)} \mathrm{d}V} = \frac{4\pi \int_0^{R(t)} v_{\mathrm{rad}}(r) r^2 \mathrm{d}r}{\frac{4}{3}\pi R^3(t)} = \frac{\alpha' \pi R^4(t)}{\frac{4}{3}\pi R^3(t)} = \frac{3}{4}\alpha' R_0 \exp(\alpha' t). \tag{17}$$

where $V(t)$ is the sphere with radius $R(t)$ at time $t$. This reveals that the average radial velocity still shows an exponential increase with time, only reduced to a factor of 3/4 (which is simply the average distance from the center in a unit sphere) with respect to the maximum radial velocity at the surface at that time.

## III. NUMERICAL SIMULATIONS

### A. Simulation framework

For our simulations, we used InPartS, a custom software package for agent-based simulations of systems of interacting particles. Implemented in the Julia programming language [8], InPartS provides a framework for quickly developing and simulating models of particles with pairwise interactions. The source code of the latest public version of InPartS, as well as further documentation and example code can be found in [9].

### B. Model implementation

The model implementation is part of our collection of related models of growing and dividing particles, published at `http://hdl.handle.net/21.11101/0000-0007-FE13-6`, and shares code with the models used in our previous work [1, 10, 11].

The equations of motion are integrated using a simple Euler integrator. Simulation time steps are selected adaptively, using a computationally cheap heuristic to estimate the maximum velocity from the computed interaction forces. The length of the next time step is then chosen to keep all displacements below 0.001 length units.

### C. Setup and procedures for simulations

Simulations are set up as described in the main text, using eight cells of random growth progress and orientation arranged on the vertices of a cube with a side length of 2 node diameters. Simulations run for 12 generations, with snapshots of the simulation state written to disk every 0.01 time units.

All random numbers used in a simulation are drawn from a seeded random number generator to provide some level of reproducibility.

Specific example code for simulations and data analysis methods used for this publication is available at `http://hdl.handle.net/21.11101/0000-0007-FE41-2`.

## IV. ANALYSIS TOOLS

### A. Sampling strategies for comparisons of simulations with different RNG seeds

Each individual parameter set is simulated with its own seed for the random number generator. The random numbers affect each cell's growth rate and hence the cell number at the end of the simulation, which is expected to be $2^{15}$ on average, but can deviate given the randomness of growth rates. We notice that, for many quantities, e.g., the average tangential velocity displayed as a function of the motility parameter, the noise in this curve is correlated with the deviations of the final cell number from the expectation value. To correct this, we could run simulations with much more than one realization for each parameter set. To save a significant increase in computational effort, we instead find the minimum number of cells at

the end of all simulations of all parameter sets, and pick a smaller number as our desired final cell number which we want to keep fixed, here: $n_{\max} = 23171$ cells. This is the expected cell number after 11.5 generations. We then find for each individual simulation the time $t_{\max}$ at which $n_{\max} = 23171$ is reached. For the best possible comparison, we usually limit our analysis to a window of 10 time units before $t_{\max}$, for each simulation. The temporal evolution of the cell number, aligned at this time, is shown in Supp. Fig. S1.

### B. Radius determination

To define the radius of the cell colony, we first compute the cell number density in equidistant spherical shells of radial thickness 0.5. We find the radius by linear interpolation between the distances between which the cell number density falls below a threshold which we set as $\rho_\Theta = 1/2\ \rho_{\text{ref}}$ where $\rho_{\text{ref}}$ is the density inside a reference volume of radius 5 after 10 generations.

### C. Velocity decomposition and tangential displacements

The dynamical variables of all cells in the system are saved in snapshots every 0.01 time units. To obtain smooth velocities, we compute them by considering the difference in positions between the snapshots, using a central difference method.

With velocities based on snapshot differences a new problem arises: with non-zero tangential velocity, the radial direction from the center to the particle changes while moving. Without adjustments, there are radial velocity contributions to the tangential velocity vector leading to a distortion. Taking this into account, the solution is to perform a velocity decomposition in sections along the displacement vector, eventually integrating the decomposed velocities. This process is performed with 100 steps along the displacement vector. A sketch of this procedure is shown in Supp. Fig. S3.

We are not only interested in decomposed velocities at individual points in time but also in a continuous trajectory of the tangential motion which can be used for MSD or OACF calculations. To this end, we perform the following steps:

*1. Tangential displacements (3D)*

In the spirit of computing them to obtain velocities, we denote displacements with $\mathbf{v}$. At each time, we first find the total displacement vector $\mathbf{v}^{3\mathrm{D}}(t_i) = \mathbf{x}(t_{i+1}) - \mathbf{x}(t_i)$ which we project onto the current radial director $\hat{\mathbf{r}}(t_i)$ to obtain the radial displacement vector

$$\mathbf{v}^{3\mathrm{D}}_{\mathrm{rad.}}(t_i) = (\mathbf{v}(t_i) \cdot \hat{\mathbf{r}}(t_i))\ \hat{\mathbf{r}}(t_i) \tag{18}$$

which we can subtract from the total displacement vector to obtain the 3D tangential displacement vector:

$$\mathbf{v}^{3\mathrm{D}}_{\mathrm{tan.}}(t_i) = \mathbf{v}^{3\mathrm{D}}(t_i) - \mathbf{v}^{3\mathrm{D}}_{\mathrm{rad.}}(t_i). \tag{19}$$

For large scale tangential motion, the radial director is also subject of rapid change. To improve accuracy, we therefore split each displacement vector into many segments (100 when finding only the magnitude, 10 when building a trajectory, cf. following section) before performing the above-mentioned displacement for each segment.

*2. Tangential displacements (2D)*

From the 3D tangential displacements, we successively build a 2D tangential trajectory, where each 2D tangential displacement has the same magnitude as the 3D tangential displacement and the direction with respect to the previous displacement is identical, with a correction accounting for the curvature. We initialize the 2D tangential displacement vector with the magnitude of the initial 3D tangential displacement vector in the x-direction and 0 in the y-direction, i.e., $\mathbf{v}^{2\mathrm{D}}_{\mathrm{tan}}(t_0) = (||\mathbf{v}^{3\mathrm{D}}_{\mathrm{tan}}(t_0)||, 0)$. Then, in each step, we perform the following procedure: We find the 3D rotation matrix $\mathbf{R}^r$ between the radial directors of $\hat{\mathbf{r}}(t_{i-1})$ and $\hat{\mathbf{r}}(t_i)$. The rotation matrix mapping from $\mathbf{p}$ to $\mathbf{q}$ in 3D is

$$\mathbf{R}(\mathbf{p}, \mathbf{q}) = \mathbf{I} + [\mathbf{f}]_x + [\mathbf{f}]_x^2\ \frac{1-c}{||\mathbf{f}||^2} \tag{20}$$

with $\mathbf{f} = \mathbf{p}\times\mathbf{q}$, $c = \mathbf{p}\cdot\mathbf{q}$ and the skew-symmetric cross-product matrix $[\mathbf{f}]_x = \begin{bmatrix} 0 & -f_3 & f_2 \\ f_3 & 0 & -f_1 \\ -f_2 & f_1 & 0 \end{bmatrix}$.

We apply $\mathbf{R}^r = \mathbf{R}(\hat{\mathbf{r}}(t_{i-1}), \hat{\mathbf{r}}(t_i))$ to the previous tangential displacement direction vector to get the current baseline vector:

$$\hat{\mathbf{b}}(t_i) = \mathbf{R}^r \frac{\mathbf{v}_{\tan}^{3\mathrm{D}}}{||\mathbf{v}_{\tan}^{3\mathrm{D}}||} \tag{21}$$

This baseline vector serves as a reference direction, taking into account curvature. The magnitude of the tangential displacement vector in 2D is simply determined by the magnitude of the tangential displacement vector in 3D. Its orientation change with respect to the previous tangential displacement vector in 2D should be equivalent to the rotation between the 3D baseline vector and the 3D tangential displacement. To ensure this, we compute the 2D rotation matrix $\mathbf{R}^v$ between the 3D baseline vector $\hat{\mathbf{b}}(t_i)$ and the 3D tangential displacement vector $\mathbf{v}_{\tan}^{3\mathrm{D}}$ under consideration of them lying in a common plane, determined by the radial director $\hat{\mathbf{r}}(t_i)$ as its normal unit vector. In general, this rotation matrix from $\hat{\mathbf{p}}$ to $\hat{\mathbf{q}}$, both 3D vectors, that lie in a plane with a normal unit vector $\hat{\mathbf{r}}$ can be calculated as the rotation by an angle $\theta$:

$$\mathbf{R}(\hat{\mathbf{p}}, \hat{\mathbf{q}}, \hat{\mathbf{r}}) = \begin{pmatrix} \cos\theta & -\sin\theta \\ \sin\theta & \cos\theta \end{pmatrix} \tag{22}$$

with

$$\theta = \mathrm{sgn}\left((\hat{\mathbf{p}} \times \hat{\mathbf{q}}) \cdot \hat{\mathbf{r}}\right) \ \arccos(\hat{\mathbf{p}} \cdot \hat{\mathbf{q}}) \tag{23}$$

We apply this rotation matrix $\mathbf{R}^v = \mathbf{R}(\hat{\mathbf{b}}(t_i), \mathbf{v}_{\tan}^{3\mathrm{D}}(t_i), \hat{\mathbf{r}}(t_i))$ on the direction of the previous 2D tangential displacement vector $\mathbf{v}_{\tan}^{2\mathrm{D}}(t_{i-1})$. We multiply with the desired magnitude and obtain the 2D tangential displacement vector $\mathbf{v}_{\tan}^{2\mathrm{D}}(t_i)$:

$$\mathbf{v}_{\tan}^{2\mathrm{D}}(t_i) = ||\mathbf{v}_{\tan}^{3\mathrm{D}}|| \ \mathbf{R}^v \frac{\mathbf{v}_{\tan}^{2\mathrm{D}}(t_{i-1})}{||\mathbf{v}_{\tan}^{2\mathrm{D}}(t_{i-1})||} \tag{24}$$

A trajectory in the 2D space is obtained by accumulating the 2D tangential displacements. We verify the procedure on the path of a trirectangular triangle on the sphere, shown in Supp. Fig. S4. Example trajectories for different motility values are shown in Supp. Fig. S5. We use these trajectories both for the calculation of mean squared displacements (MSDs) and orientation autocorrelation functions (OACFs). Except for the fraction $f_{\text{in}}$ of inwards

moving cells that uses the sign of the instantaneous radial speed, only velocities obtained by snapshot differences are used in the analysis.

### D. Mixing efficiency

At time $t_0$, we consider cells in a spherical sample volume $s$ with a radius of $f_{\mathrm{SV}} = \frac{1}{3}$ of the radius of the colony, positioned at a distance of $\frac{1}{2}$ of the radius of the colony from the center. For a lag time $\Delta t$, we track the positions of these cells and their descendants, both referred to as $D(s)$, to obtain a qualitative and quantitative image of how they move within the colony. We propose a measure to differentiate between cells staying within their neighborhood, i.e., within the sample volume, considering its growth along with the overall growth of the colony, and cells being able to escape their confinement among neighbors and explore the entire colony. We argue that the average distance from the mean positions of the tracked cells, normalized by the radius of the sample volume, is an appropriate measure. For all cells in a sample volume we compute the distance from their average position $\bar{\mathbf{r}}$ and then average over all obtained distances. We normalize this by the radius of a sample volume $f_{\mathrm{SV}} \cdot R$ under assumption that it grows along with the overall colony growth, i.e., considering the current $R$. Considering cells in one sample volume $s$, we obtain

$$\tilde{\eta}_M(t_0, \Delta t) = \frac{\langle ||\mathbf{r} - \bar{\mathbf{r}}|| \rangle}{f_{\mathrm{SV}} \cdot R}, \tag{25}$$

where all quantities on the right except the parameter $f_{\mathrm{SV}}$ depend on time and are measured at $t_0 + \Delta t$. For better statistics, we consider not only one sample volume, but a set $S$ of six sample volumes $s$ of radius $f_{\mathrm{SV}} = \frac{1}{3}$ sitting along the three spatial axes at $\left(\pm\frac{1}{2}, 0, 0\right)$, $\left(0, \pm\frac{1}{2}, 0\right)$, $\left(0, 0, \pm\frac{1}{2}\right)$ in the system of the colony. In this case, we compute $\tilde{\eta}_M$ by collecting all distances of cells from the average position in their respective sample volume and then average over these distances. In the edge case of complete confinement, cells stay within the growing sample volume of radius $f_{\mathrm{SV}} \cdot R$. In the case of complete mixing, the cells are within a volume of radius $R$. The average distance in a sphere with radius $R$ to its center is

$$\left(\frac{4}{3}\pi R^3\right)^{-1} \int_V r \; \mathrm{d}V = \frac{3}{4} R. \tag{26}$$

Consequently, $\tilde{\eta}_M = \frac{3}{4f_{\rm SV}}$ in the case of perfect mixing and $\tilde{\eta}_M = \frac{3}{4}$ in the case of confinement. These are the edge cases of this measure. We normalize

$$\eta_M(t_0, \Delta t) = \frac{4 \cdot f_{\rm SV}}{3 \cdot (1 - f_{\rm SV})} \frac{\langle ||\mathbf{r} - \bar{\mathbf{r}}|| \rangle}{f_{\rm SV} \cdot R} - \frac{f_{\rm SV}}{(1 - f_{\rm SV})}, \tag{27}$$

to obtain the mixing efficiency $\eta_M$ which yields 1 and 0 for these two cases, respectively. For $f_{\rm SV} = \frac{1}{3}$, this reduces to

$$\eta_M(t_0, \Delta t) = \frac{2}{R} \langle ||\mathbf{r}_c - \bar{\mathbf{r}}|| \rangle - \frac{1}{2}. \tag{28}$$

### E. Mixing efficiency contour line and mixing time scale fit

We plot the contour line using *matplotlib.pyplot.contour* [12] that also provides data points of the contour line. We then perform a fit of the form

$$\Delta t|_{\eta_M = 1/2}(M) = A \cdot (M - M_\infty)^\beta + C, \tag{29}$$

finding $A \approx 960$, $\beta \approx -1.08$, $C \approx 0.18$, and most interestingly, $M_\infty \approx 900$ (compare Supp. Fig. S11).

### F. Diffusion of a uniform sphere on a growing domain

For our phenomenological model, we consider the cells of the sample volume to perform a persistent random walk. We want to describe this as the dynamics of free particles following a diffusion equation

$$\frac{\partial P(\mathbf{r}, t)}{\partial t} = D \nabla^2 P(\mathbf{r}, t) \tag{30}$$

where $P(\mathbf{r}, t)$ represents the probability density function. For now, the origin of this diffusion process is not of interest. The heat kernel, the Green's function of the diffusion equation, reads

$$G(\mathbf{r}, t) = \frac{1}{(4\pi D t)^{3/2}} \exp\left( - \frac{||\mathbf{r}||^2}{4Dt} \right) \tag{31}$$

As initial condition, we assume a uniform sphere of radius $Q$

$$P(\mathbf{r},0) = \begin{cases} \left(\frac{4}{3}\pi Q^3\right)^{-1} & ,r \leq Q \\ 0 & ,\text{else} \end{cases} \tag{32}$$

Convolving the initial condition with the heat kernel yields

$$P(r,t) = \frac{3}{8\pi Q^3}\left[\operatorname{erf}\left(\frac{r+Q}{\sqrt{u}}\right) - \operatorname{erf}\left(\frac{r-Q}{\sqrt{u}}\right) + \frac{\sqrt{u}}{\sqrt{\pi}r}\left(\exp\left(-\frac{(r+Q)^2}{u}\right) - \exp\left(-\frac{(r-Q)^2}{u}\right)\right)\right], \tag{33}$$

where $u = 4Dt$, a result that can also be found in literature [13–15]. Here, $\operatorname{erf}(\cdot)$ is the error function. The time series of the relative spread can be obtained by computing the temporal evolution of the mean of the probability density function:

$$\langle r\rangle(t) = \iiint_V rP(r,t)\ \mathrm{d}V = \frac{3}{8Q^3}\left(\frac{\sqrt{u}Q(u+2Q^2)}{\sqrt{\pi}\exp\left(\frac{Q^2}{u}\right)} - \frac{u^2-4uQ^2-4Q^4}{2}\operatorname{erf}\left(\frac{Q}{\sqrt{u}}\right)\right) \tag{34}$$

. We can verify the limits $\lim_{t\to 0^+}\langle r\rangle(t) = \frac{3}{4}Q$, which is the average distance from the center of the initial sphere, and $\lim_{t\to\infty}\frac{\langle r\rangle(t)}{\sqrt{(t)}} = \frac{4\sqrt{D}}{\sqrt{\pi}}$, which is the long term behavior of diffusion of a point source. To account for exponential growth of the domain, we rewrite the diffusion equation

$$\frac{\partial P}{\partial t} = D\frac{\partial^2 P}{\partial \tilde{r}^2} \tag{35}$$

with $\tilde{r} = \exp(\alpha' t)$. Since $\frac{\partial}{\partial \tilde{r}} = \frac{\partial}{\partial r}\frac{\partial r}{\partial \tilde{r}} = \exp(-\alpha' t)\frac{\partial}{\partial r}$, we can write $\frac{\partial^2}{\partial \tilde{r}^2} = \exp(-2\alpha' t)\frac{\partial^2}{\partial r^2}$ and hence

$$\frac{\partial P}{\partial \tilde{t}} = D\frac{\partial^2 P}{\partial r^2} \tag{36}$$

if the condition $\frac{\partial}{\partial \tilde{t}} = \exp(-2\alpha' t)\frac{\partial}{\partial t}$ is fulfilled, which is the case when $\frac{\partial \tilde{t}}{\partial t}$. As a consequence, we can find the suitable time scale transform that has the same effect as the initially introduced length scale transform:

$$\tilde{t} = \int_0^t \mathrm{d}\tau \exp(-2\alpha'\tau) = \frac{1}{2\alpha'}\left(1 - \exp(-2\alpha' t)\right) \tag{37}$$

Applying this transform to the relative spread $\langle r\rangle$, we can consequently compute the mixing efficiency $\eta_M$, assuming an initial sample volume with radius $Q = R_*/3$. Instead of $R(t)$, we

can normalize by $R_*$, given that the exponential expansion (and subsequent renormalization to the initial radius) is already included in the time transform. It should be noted that this phenomenological description of free diffusion allows for a spreading of density beyond a radius of $3Q = R_*$, which is not possible in our simulations where cells from the sample volume cannot leave the spheroid. However, if we only consider mixing up to $\eta_M = 1/2$, we can verify that, in the cases we consider, less that 1% of the probability density diffuses beyond the distance where the boundary of the spheroid would be.

### G. Long term diffusion of tumbling athermal active Brownian particles

The following derivation closely follows the considerations on intermittently self-propelling particles by Datta et al. [16]. We use their main result (Eq. 16) to obtain the velocity autocorrelation $\hat{\hat{C}}_{vv}(s,u)$ in Laplace space. We consider an athermal ABP with rotational diffusion $D_r$ that additionally exhibits tumbles in a random direction (hence $\langle \cos\chi \rangle = 0$). We do not consider turn phases, hence $\psi_t = 0$ and consequently $\hat{\psi}_t = 1$. Under these constraints, the velocity autocorrelation in Laplace space, for arbitrary run time distributions $\psi_r(t)$ reads

$$\hat{\hat{C}}_{vv}(s,u) = \frac{v^2}{u + D_r}\left(\frac{1}{s} - \frac{\hat{\psi}_r(u + D_r) - \hat{\psi}_r(s)}{(s - u - D_r)(1 - \hat{\psi}_r(s))}\right) \tag{38}$$

Using Eqs. 7 and 8 from [16], adjusted for 3D, we can find the long term diffusion coefficient as a function of the intra-generational persistence time $\tau_r = D_r^{-1}$:

$$D = \frac{1}{3}\lim_{u\to 0}\ \lim_{s\to 0} s\ \hat{\hat{C}}_{vv}(s,u) = \frac{1}{3}\frac{v^2}{D_r}(1 - \Omega) = \frac{1}{3}v^2\tau_r(1 - \Omega) \tag{39}$$

We notice that the long term diffusivity still has the same form as for the classic athermal ABP, with an effective persistence time $\tau_{\text{eff}} = \tau_r(1 - \Omega)$, that is only corrected by $\Omega$, which is to be calculated as

$$\Omega = \lim_{s\to 0} \frac{s\left(\hat{\psi}_r(1/\tau_r) - \hat{\psi}_r(s)\right)}{(s - 1/\tau_r)\cdot\left(1 - \hat{\psi}_r(s)\right)} = \lim_{s\to 0}\frac{\Omega_1}{\Omega_2} \tag{40}$$

We can easily see that $\lim_{s\to 0}\Omega_1 = 0$. Also since $\hat{\psi}_r(0) = 1$, by definition of the Laplace transform of a probability density, $\lim_{s\to 0}\Omega_2 = 0$. With the limits of numerator $\Omega_1$ and

denominator $\Omega_2$ both being 0, we have to apply L'Hôpital's rule to find $\Omega$:

$$\Omega = \lim_{s\to 0} \frac{\mathrm{d}\Omega_1/\mathrm{d}s}{\mathrm{d}\Omega_2/\mathrm{d}s} \tag{41}$$

$$= \lim_{s\to 0} \frac{\hat{\psi}_r(1/\tau_r) - \hat{\psi}_r(s) - s\cdot \mathrm{d}\hat{\psi}_r(s)/\mathrm{d}s}{1 + (1/\tau_r - s)\cdot \mathrm{d}\hat{\psi}_r(s)/\mathrm{d}s - \hat{\psi}_r(s)} \tag{42}$$

$$= \frac{\hat{\psi}_r(1/\tau_r) - 1}{1/\tau_r \cdot \lim_{s\to 0} \mathrm{d}\hat{\psi}_r(s)/\mathrm{d}s}. \tag{43}$$

Hence, the final result for the diffusion constant only requires the explicit form of $\hat{\psi}_r(s)$ as well as its derivative with respect to $s$:

$$D = \frac{1}{3}v^2\tau_r \left(1 + \frac{\tau_r\cdot\left(1 - \hat{\psi}_r(1/\tau_r)\right)}{\lim_{s\to 0}\mathrm{d}\hat{\psi}_r(s)/\mathrm{d}s}\right) \tag{44}$$

First, we consider the very simple case of a fixed run time $T$ between tumbles, hence $\psi_r(t) = \delta(t-T)$ and in Laplace space $\hat{\psi}_r(s) = \exp(-sT)$, with derivative $\mathrm{d}\hat{\psi}_r(s)/\mathrm{d}s = -T\exp(-sT)$ and $\lim_{s\to 0}\mathrm{d}\hat{\psi}_r(s)/\mathrm{d}s = -T$. As a result:

$$D = \frac{1}{3}v^2\tau\left(1 - \frac{\tau}{T}\left(1 - \exp\left(-\frac{T}{\tau}\right)\right)\right). \tag{45}$$

We can also calculate an expression for $D$ considering the true run time between reorientations at cell division. A comparison with the much simpler case that is presented here is shown in Supp. Fig. S13.

### H. Comparison with velocities in experiments

In our analysis, we find a typical critical velocity of $v_\infty \approx 9$ cell diameters per generation. This is a tangential velocity, the according magnitude under the assumption of isotropic non-affine velocities is stretched by $4/\pi$, resulting in a typical critical velocity around 11.5 cell diameters per generation. There is little to no research on cell velocities in vivo or in spheroids before and after the EMT, hence we consider a study by Quinsgaard et al. [17] where lineage speeds of MDA-MB-468 breast cancer cells before and after the EGF-induced EMT are measured. We estimate the speed of the control group as $v_{\mathrm{control}} = (7\pm 3)$ µm h$^{-1}$

and the speed of cells treated with 50 ng mL$^{-1}$ EGF as $v_{\mathrm{EGF50}} = (15 \pm 5)$ µm h$^{-1}$. From their microscopy images we infer a typical cell size of $(20 \pm 5)$ µm. We assume a doubling time of $(40 \pm 10)$ h, extracted from growth curves of the control group. We are aware that cell growth is inhibited after the EMT, but still aim for a velocity in terms of generations before the EMT. As a result, we find typical speeds to be $(14 \pm 8)$ cell diameters per generation before the EMT and $(30 \pm 15)$ cell diameters per generation after the EMT.

## V. SUPPLEMENTAL FIGURES

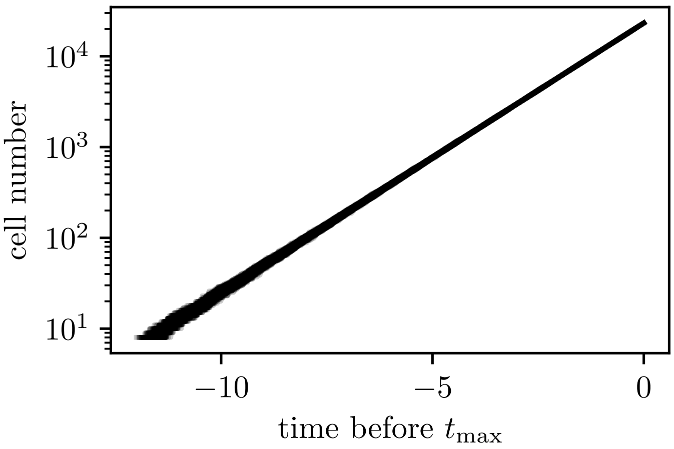


Supp. Fig. S1. Temporal evolution of the total cell number in all simulations of motility and growth rate scans, aligned at $t_{\mathrm{max}}$, the individual time when $N_{\mathrm{max}}$ is reached.

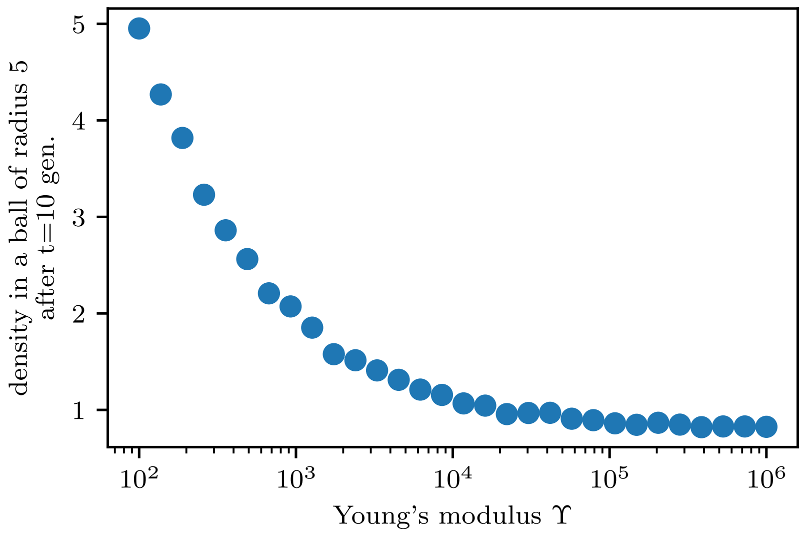


SUPP. FIG. S2. The density in a sample ball after 10 generations of simulation as a function of the Young's modulus $\Upsilon$ clearly shows convergence to an incompressible limit. This justifies our choice of $\Upsilon = 10^5$.

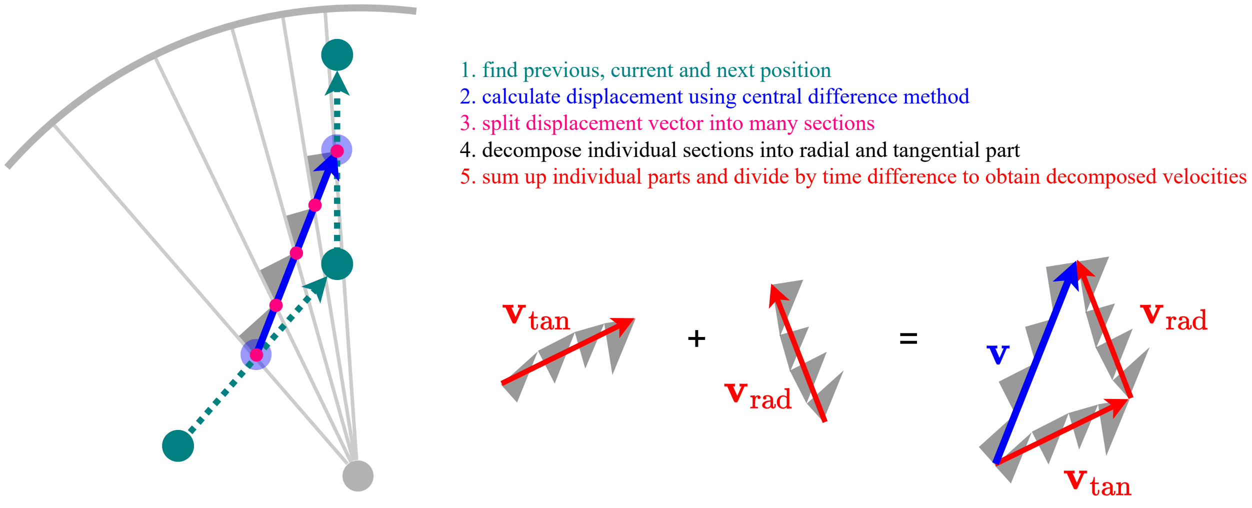


SUPP. FIG. S3. Schematic representation of the velocity decomposition into radial and tangential component that takes into account the change of the radial direction along the displacement vector.

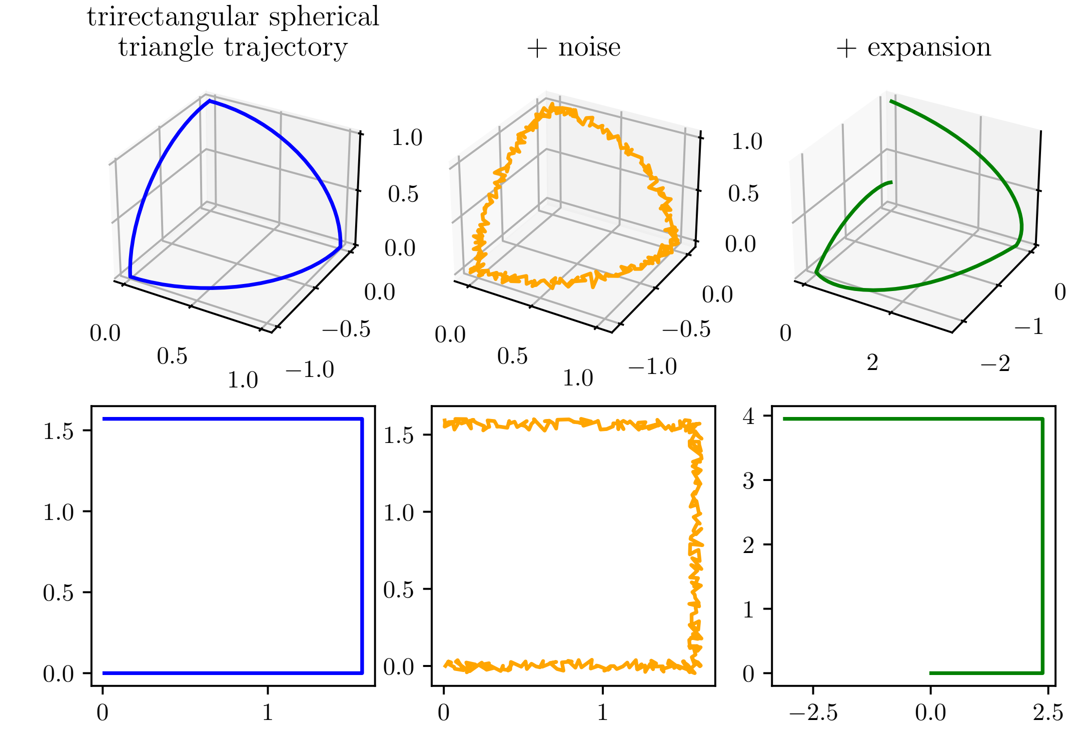


SUPP. FIG. S4. Demonstration of the decomposition of trirectangular trajectories on a spherical surface with extensions (noise and expansion) to 2D tangential trajectories.

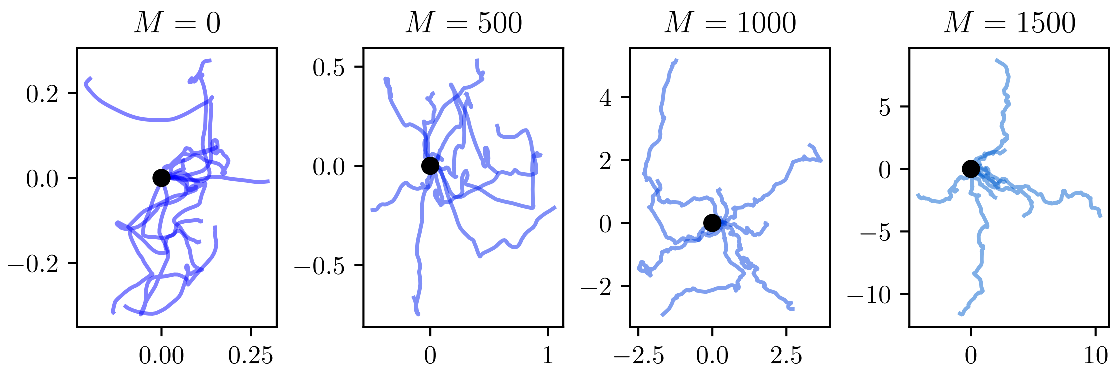


SUPP. FIG. S5. Examples for 2D tangential trajectories using data between cell divisions for different motility values. The orientation of all trajectories is chosen such that the initial displacement goes to the right from the black starting point. The shown trajectories are selected to last at least 0.8 generations.

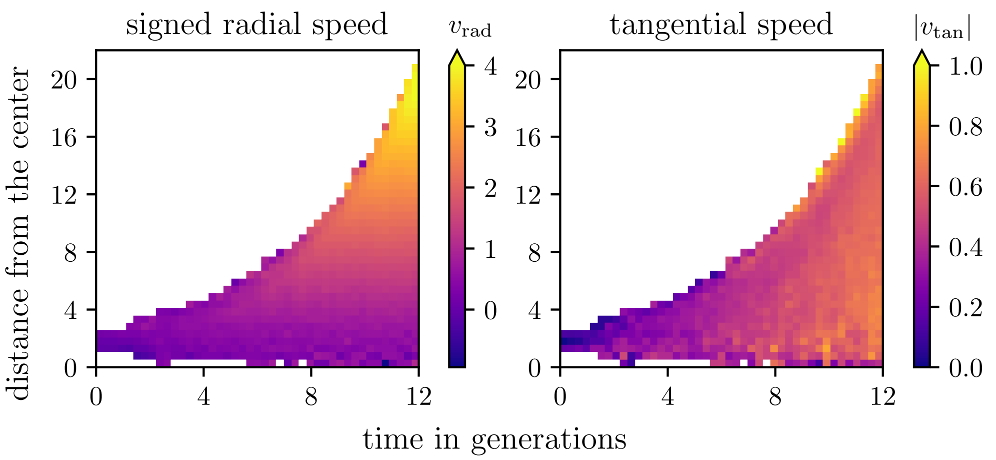


Supp. Fig. S6. Radial and tangential velocities as function of time and distance from the center, averaged over the tangential direction.

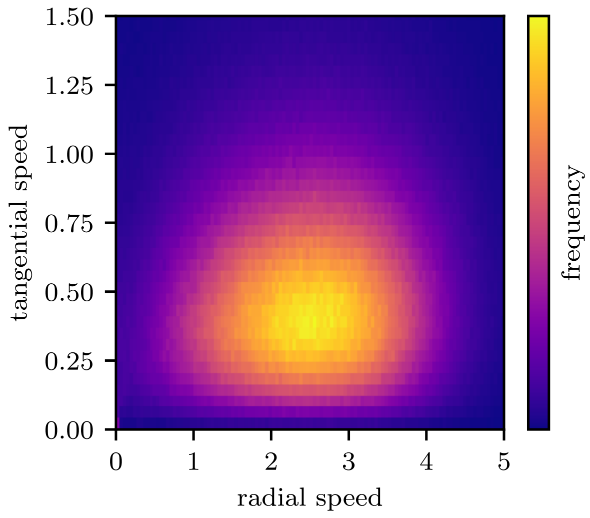


Supp. Fig. S7. Radial and tangential velocities of individual cells in the spheroid are uncorrelated.

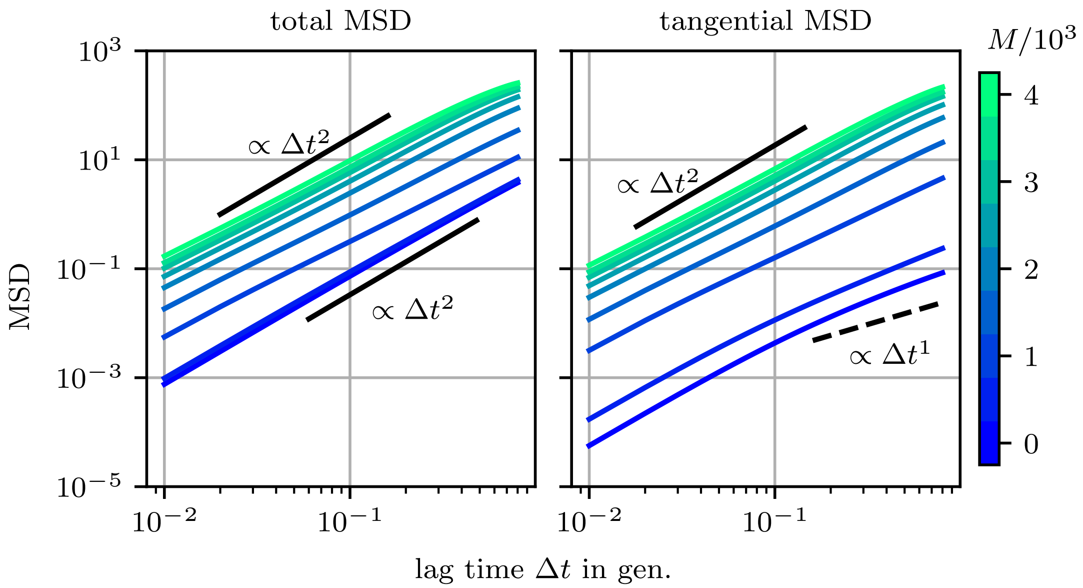


SUPP. FIG. S8. Comparison of the total and tangential MSD for different values of the motility parameter $M$ with a focus on their slope in log-log representation.

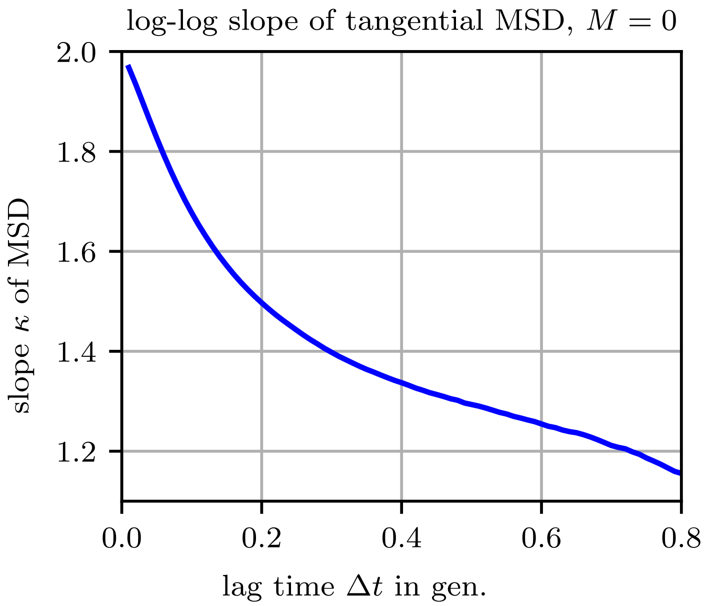


SUPP. FIG. S9. Slope of the tangential MSD over lag time, taken from a log-log plot, indicating approximately diffusive motion towards longer lag times in the non-motile case ($M = 0$).

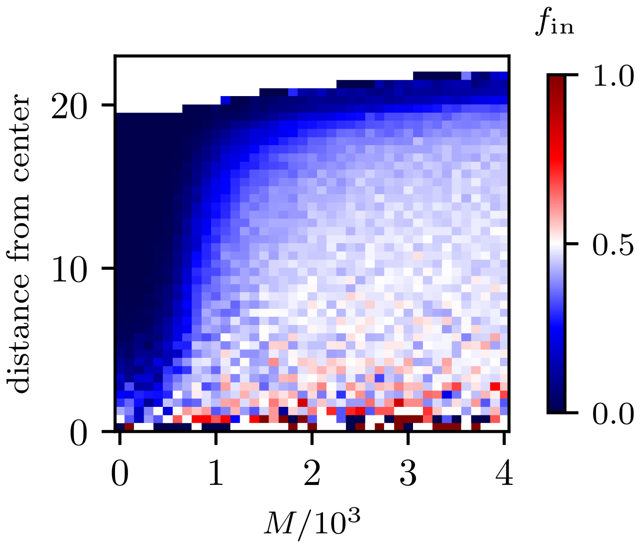


Supp. Fig. S10. Spatial distribution of the fraction of radially inwards moving cells for different motilities, after $t = t_{\mathrm{max}}$, averaged over the tangential direction, taking into account instantaneous velocities.

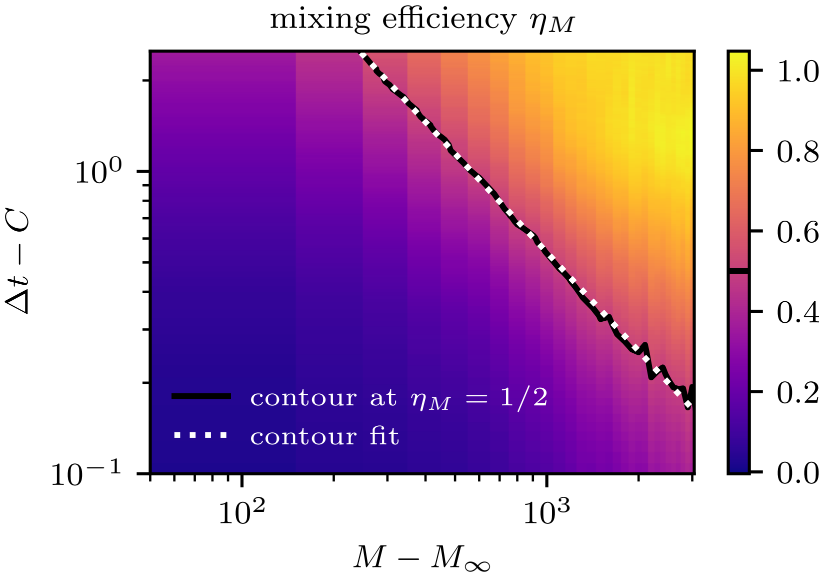


Supp. Fig. S11. Log-log representation of the $\eta_M = 1/2$ contour line and its fit, suggesting a shifted hyperbola.

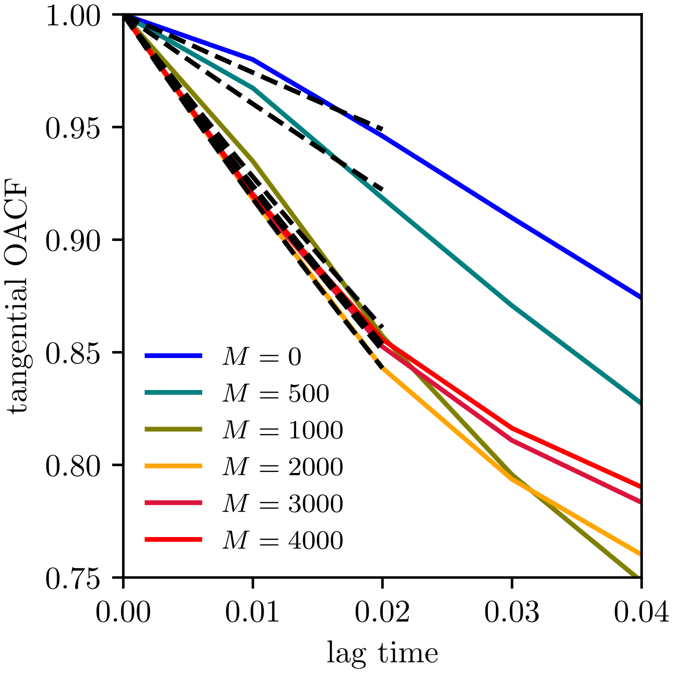


SUPP. FIG. S12. Exponential fits to the initial decay of the tangential orientation autocorrelation function $\text{OACF}(\Delta t) = \langle \hat{\mathbf{v}}_c(t_0) \cdot \hat{\mathbf{v}}_c(t_0 + \Delta_t) \rangle_{t_0,c}$, computed from trajectories between division events.

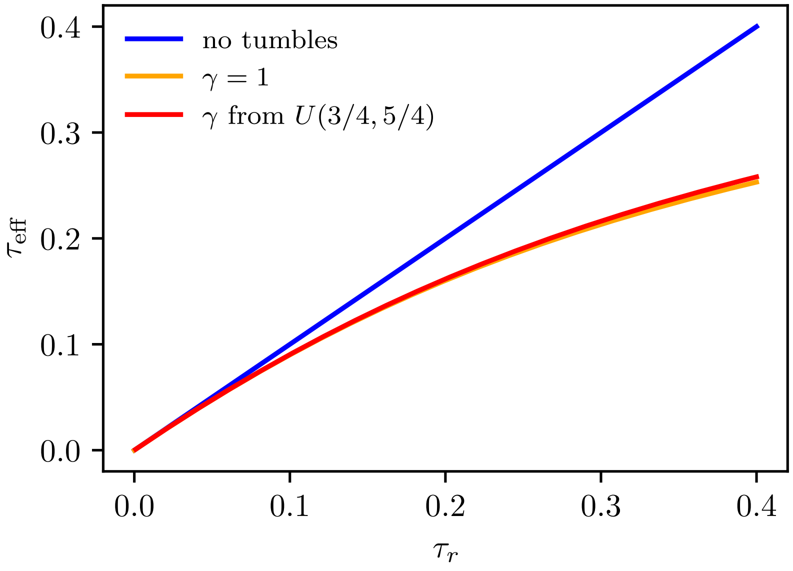


SUPP. FIG. S13. Relation between the persistence time $\tau_r$ of orientation between tumbles and the effective persistence time including tumbles with different distributions of the run time between tumbles. As a simplification, the result for a delta-distributed run time of 1 is almost indistinguishable from the result that considers the true growth rate distribution in our simulations, where the inverse of the run time is drawn from a uniform distribution between 3/4 and 5/4.

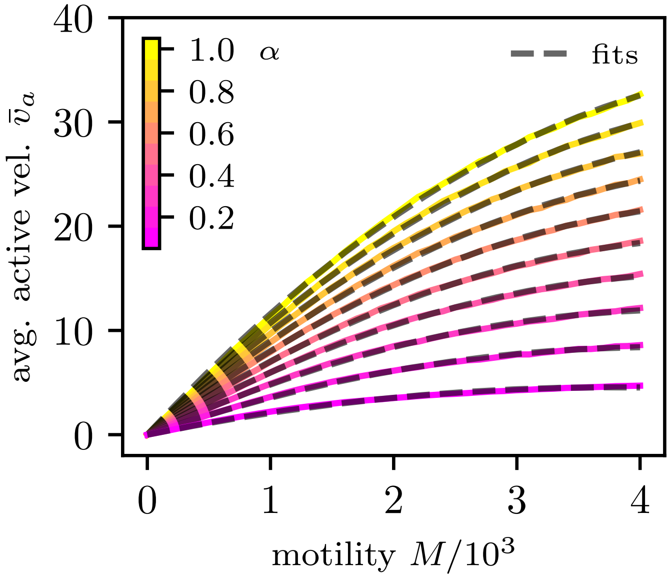


Supp. Fig. S14. Relation between the average active velocity and the motility parameter with parabola fits (dashed lines), which capture the data extremely well and used for converting between $M$ and $\bar{v}_a$ without being affected by noise.

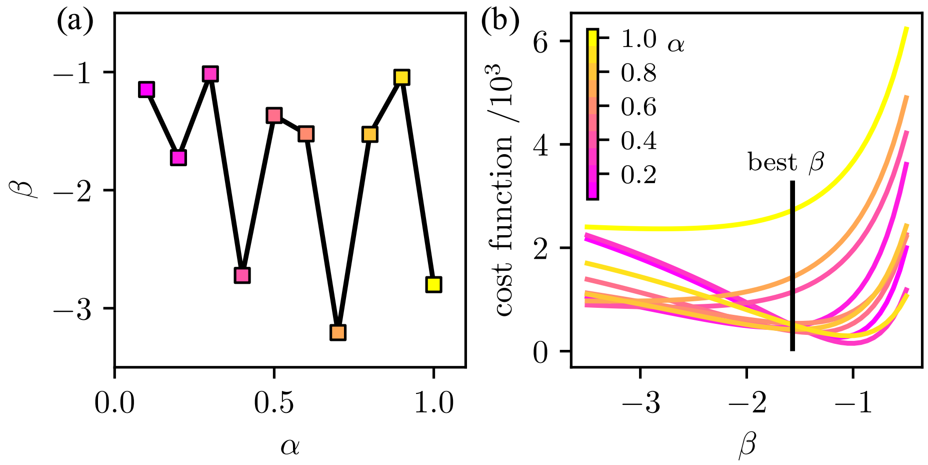


Supp. Fig. S15. Fitting data in Fig. 6b to determine critical active velocity for different bulk doubling rates $\alpha$. (a) The fit parameter $\beta$ from individual fits of the mixing efficiency contour lines is noisy with no discernable trend. We therefore suspect that $\beta$ is not very well constrained, making it sensitive to random fluctuations in the data. (b) Fitting all hyperbolas simultaneously with one global $\beta$ (but different critical velocities) yields an optimal value of $-1.57$. Indeed, the landscape of the cost function, i.e., mean squared residual between fit and data, is rather shallow in the vicinity of this value, especially in the cases where a very negative $\beta$ was the optimal choice. The critical values of $\bar{v}_a$ at which the time scale of mixing diverges, which are plotted in Fig. 6c, are therefore obtained using the global-$\beta$ fit strategy.

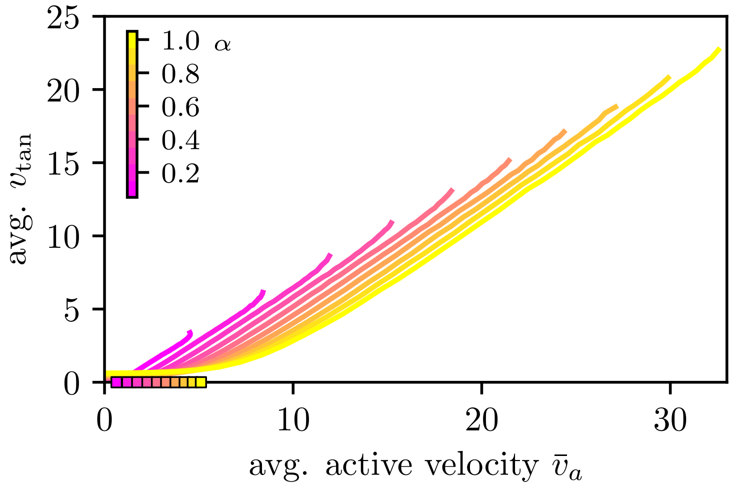


SUPP. FIG. S16. Average tangential speed as in Fig. 5d (purple line), but as a function of the average active velocity and for different bulk doubling rates $\alpha$. We define the onset of the tangential speed as the motility at which the avg. $v_{\tan}$ has increased by more than 20% of its initial value at $\bar{v}_a = 0$ (squares).

## VI. SUPPLEMENTAL VIDEOS

**V1:** An exponentially growing spheroidal cell colony in the case of no additional cell motility ($M = 0$). This movie shows proliferation over a time of 12 generations. Cell colors indicate their current growth progress, from light to dark teal.

**V2-V5:** Mixing of a sample volume within the spheroid. After a time of $t_{\mathrm{max}} - 3$ gen., cells inside a spherical sample volume are marked in red, with the brightness again indicating their growth progress. These cells and their descendants are tracked and marked over a lag time of $\Delta t = 3$ gen. until $t_{\mathrm{max}}$. The other cells are made transparent. The movies show different behavior for different cell motility: Cells stay confined in their neighborhood for no motility ($M = 0$, V2) and low motility ($M = 500$, V3) but can escape these confinements and mix within the colony for larger motility ($M = 1000$, V4). This mixing occurs quicker with even larger motility ($M = 2000$, V5).

[1] J. Isensee, L. Hupe, R. Golestanian, and P. Bittihn, Stress anisotropy in confined populations of growing rods, Journal of The Royal Society Interface **19**, 20220512 (2022).

[2] H. Hertz, Ueber die Berührung fester elastischer Körper., Journal für die reine und angewandte Mathematik **1882**, 156 (1882).

[3] M. M. Tirado, C. L. Martínez, and J. G. de la Torre, Comparison of theories for the translational and rotational diffusion coefficients of rod-like macromolecules. application to short DNA fragments, The Journal of Chemical Physics **81**, 2047 (1984).

[4] M. M. Tirado and J. G. de la Torre, Translational friction coefficients of rigid, symmetric top macromolecules. Application to circular cylinders, The Journal of Chemical Physics **71**, 2581 (1979).

[5] M. M. Tirado and J. G. de la Torre, Rotational dynamics of rigid, symmetric top macromolecules. Application to circular cylinders, The Journal of Chemical Physics **73**, 1986 (1980).

[6] H. H. Wensink, J. Dunkel, S. Heidenreich, K. Drescher, R. E. Goldstein, H. Löwen, and J. M. Yeomans, Meso-scale turbulence in living fluids, Proceedings of the National Academy of Sciences **109**, 14308 (2012).

[7] J. Isensee, L. Hupe, R. Golestanian, and P. Bittihn, Supplementary information from Stress anisotropy in confined populations of growing rods (2022).

[8] J. Bezanson, A. Edelman, S. Karpinski, and V. B. Shah, Julia: A fresh approach to numerical computing, SIAM Review **59**, 65 (2017).

[9] L. Hupe, J. Isensee, and P. Bittihn, InPartS. Interacting particle simulations in Julia (2022).

[10] M. Stevanovic, T. Boukéké-Lesplulier, L. Hupe, J. Hasty, P. Bittihn, and D. Schultz, Nutrient Gradients Mediate Complex Colony-Level Antibiotic Responses in Structured Microbial Populations, Front. Microbiol. **13** (2022).

[11] L. Hupe, Y. G. Pollack, J. Isensee, A. Amiri, R. Golestanian, and P. Bittihn, A minimal model of smoothly dividing disk-shaped cells, arXiv , 2409.01959 (2024).

[12] J. D. Hunter, Matplotlib: A 2D graphics environment, Computing in Science & Engineering **9**, 90 (2007).

[13] H. Carslaw and J. Jaeger, *Conduction of Heat in Solids*, Oxford science publications (Clarendon Press, 1959).

[14] T. S. Lovering, Theory of heat conduction applied to geological problems, Geological Society of America Bulletin **46**, 69–94 (1935).

[15] L. Ingersoll and O. Zobel, *An Introduction to the Mathematical Theory of Heat Conduction: With Engineering and Geological Applications* (Ginn, 1913).

[16] A. Datta, C. Beta, and R. Großmann, Random walks of intermittently self-propelled particles, Physical Review Research **6**, 043281 (2024).

[17] E. M. B. Quinsgaard, M. S. Korsnes, R. Korsnes, and S. A. Moestue, Single-cell tracking as a tool for studying EMT-phenotypes, Experimental Cell Research **437**, 113993 (2024).
